# Supplementary material for: MimicGAN: Corruption-Mimicking for Blind Image Recovery & Adversarial Defense
Source: arXiv:1811.08484 source file (2018-11-20)
Supplement: Supplementary file 1 [file supplementary.tex]

\documentclass[10pt,twocolumn,letterpaper]{article}

\usepackage{cvpr}
\usepackage{times}
\usepackage{epsfig}
\usepackage{graphicx}
\usepackage{listings}
\usepackage{hyperref}
\usepackage{listings}
\usepackage{color}
\usepackage{textcomp}
\definecolor{listinggray}{gray}{1.0}
\definecolor{lbcolor}{rgb}{1.0,1.0,1.0}
\lstset{
	backgroundcolor=\color{lbcolor},
	tabsize=3,
	rulecolor=,
	language=python,
        basicstyle=\scriptsize,
        upquote=true,
        aboveskip={\baselineskip},
        columns=fixed,
        showstringspaces=false,
        extendedchars=true,
        breaklines=true,
        prebreak = \raisebox{0ex}[0ex][0ex]{\ensuremath{\hookleftarrow}},
        frame=false,
        showtabs=false,
        showspaces=false,
        showstringspaces=false,
        identifierstyle=\ttfamily,
        keywordstyle=\color[rgb]{0,0,1},
        commentstyle=\color[rgb]{0.133,0.545,0.133},
        stringstyle=\color[rgb]{0.627,0.126,0.941},
}
\usepackage{pythonhighlight}
\usepackage{amsmath}
\usepackage{amssymb}
\usepackage{textcomp}
\usepackage{subfig}
\usepackage[export]{adjustbox}
\usepackage{ctable}
\usepackage{colortbl}
\usepackage{float}
% Include other packages here, before hyperref.

% If you comment hyperref and then uncomment it, you should delete
% egpaper.aux before re-running latex.  (Or just hit 'q' on the first latex
% run, let it finish, and you should be clear).
%\usepackage[pagebackref=true,breaklinks=true,letterpaper=true,colorlinks,bookmarks=false]{hyperref}

%\cvprfinalcopy % *** Uncomment this line for the final submission
%\usepackage{authblk}

 % *** Enter the CVPR Paper ID here

% Pages are numbered in submission mode, and unnumbered in camera-ready
\ifcvprfinal\pagestyle{empty}\fi
\begin{document}

%%%%%%%%% TITLE
\title{Supplementary Material for MimicGAN}

%\author[]{Rushil Anirudh, Jayaraman J. Thiagarajan, Bhavya Khailkura, Timo Bremer}
%\affil[]{Lawrence Livermore National Laboratory.}

\maketitle
\section{CelebA Dataset}
\input{celeba.tex}
\section{Fashion-MNIST Dataset}
\input{mnist.tex}

\small{
\bibliographystyle{ieee}
\bibliography{refs}
}

\end{document}
